# Supplementary material for: Validation of a simulation model for FaaS performance benchmarking using predictive validation
Source: arXiv:2106.15555 source file (2021-06-29)
Supplement: Supplementary file 1 [file 15-appendice.tex]

\section{Appendices}

If your work needs an appendix, add it before the
``\verb|\end{document}|'' command at the conclusion of your source
document.

Start the appendix with the ``\verb|appendix|'' command:
\begin{verbatim}
  \appendix
\end{verbatim}
and note that in the appendix, sections are lettered, not
numbered. This document has two appendices, demonstrating the section
and subsection identification method.
